# Supplementary material for: Learning Tuple Compatibility for Conditional OutfitRecommendation
Source: arXiv:2008.08189 source file (2020-08-18)
Supplement: Supplementary file 1 [file supplementary.pdf]

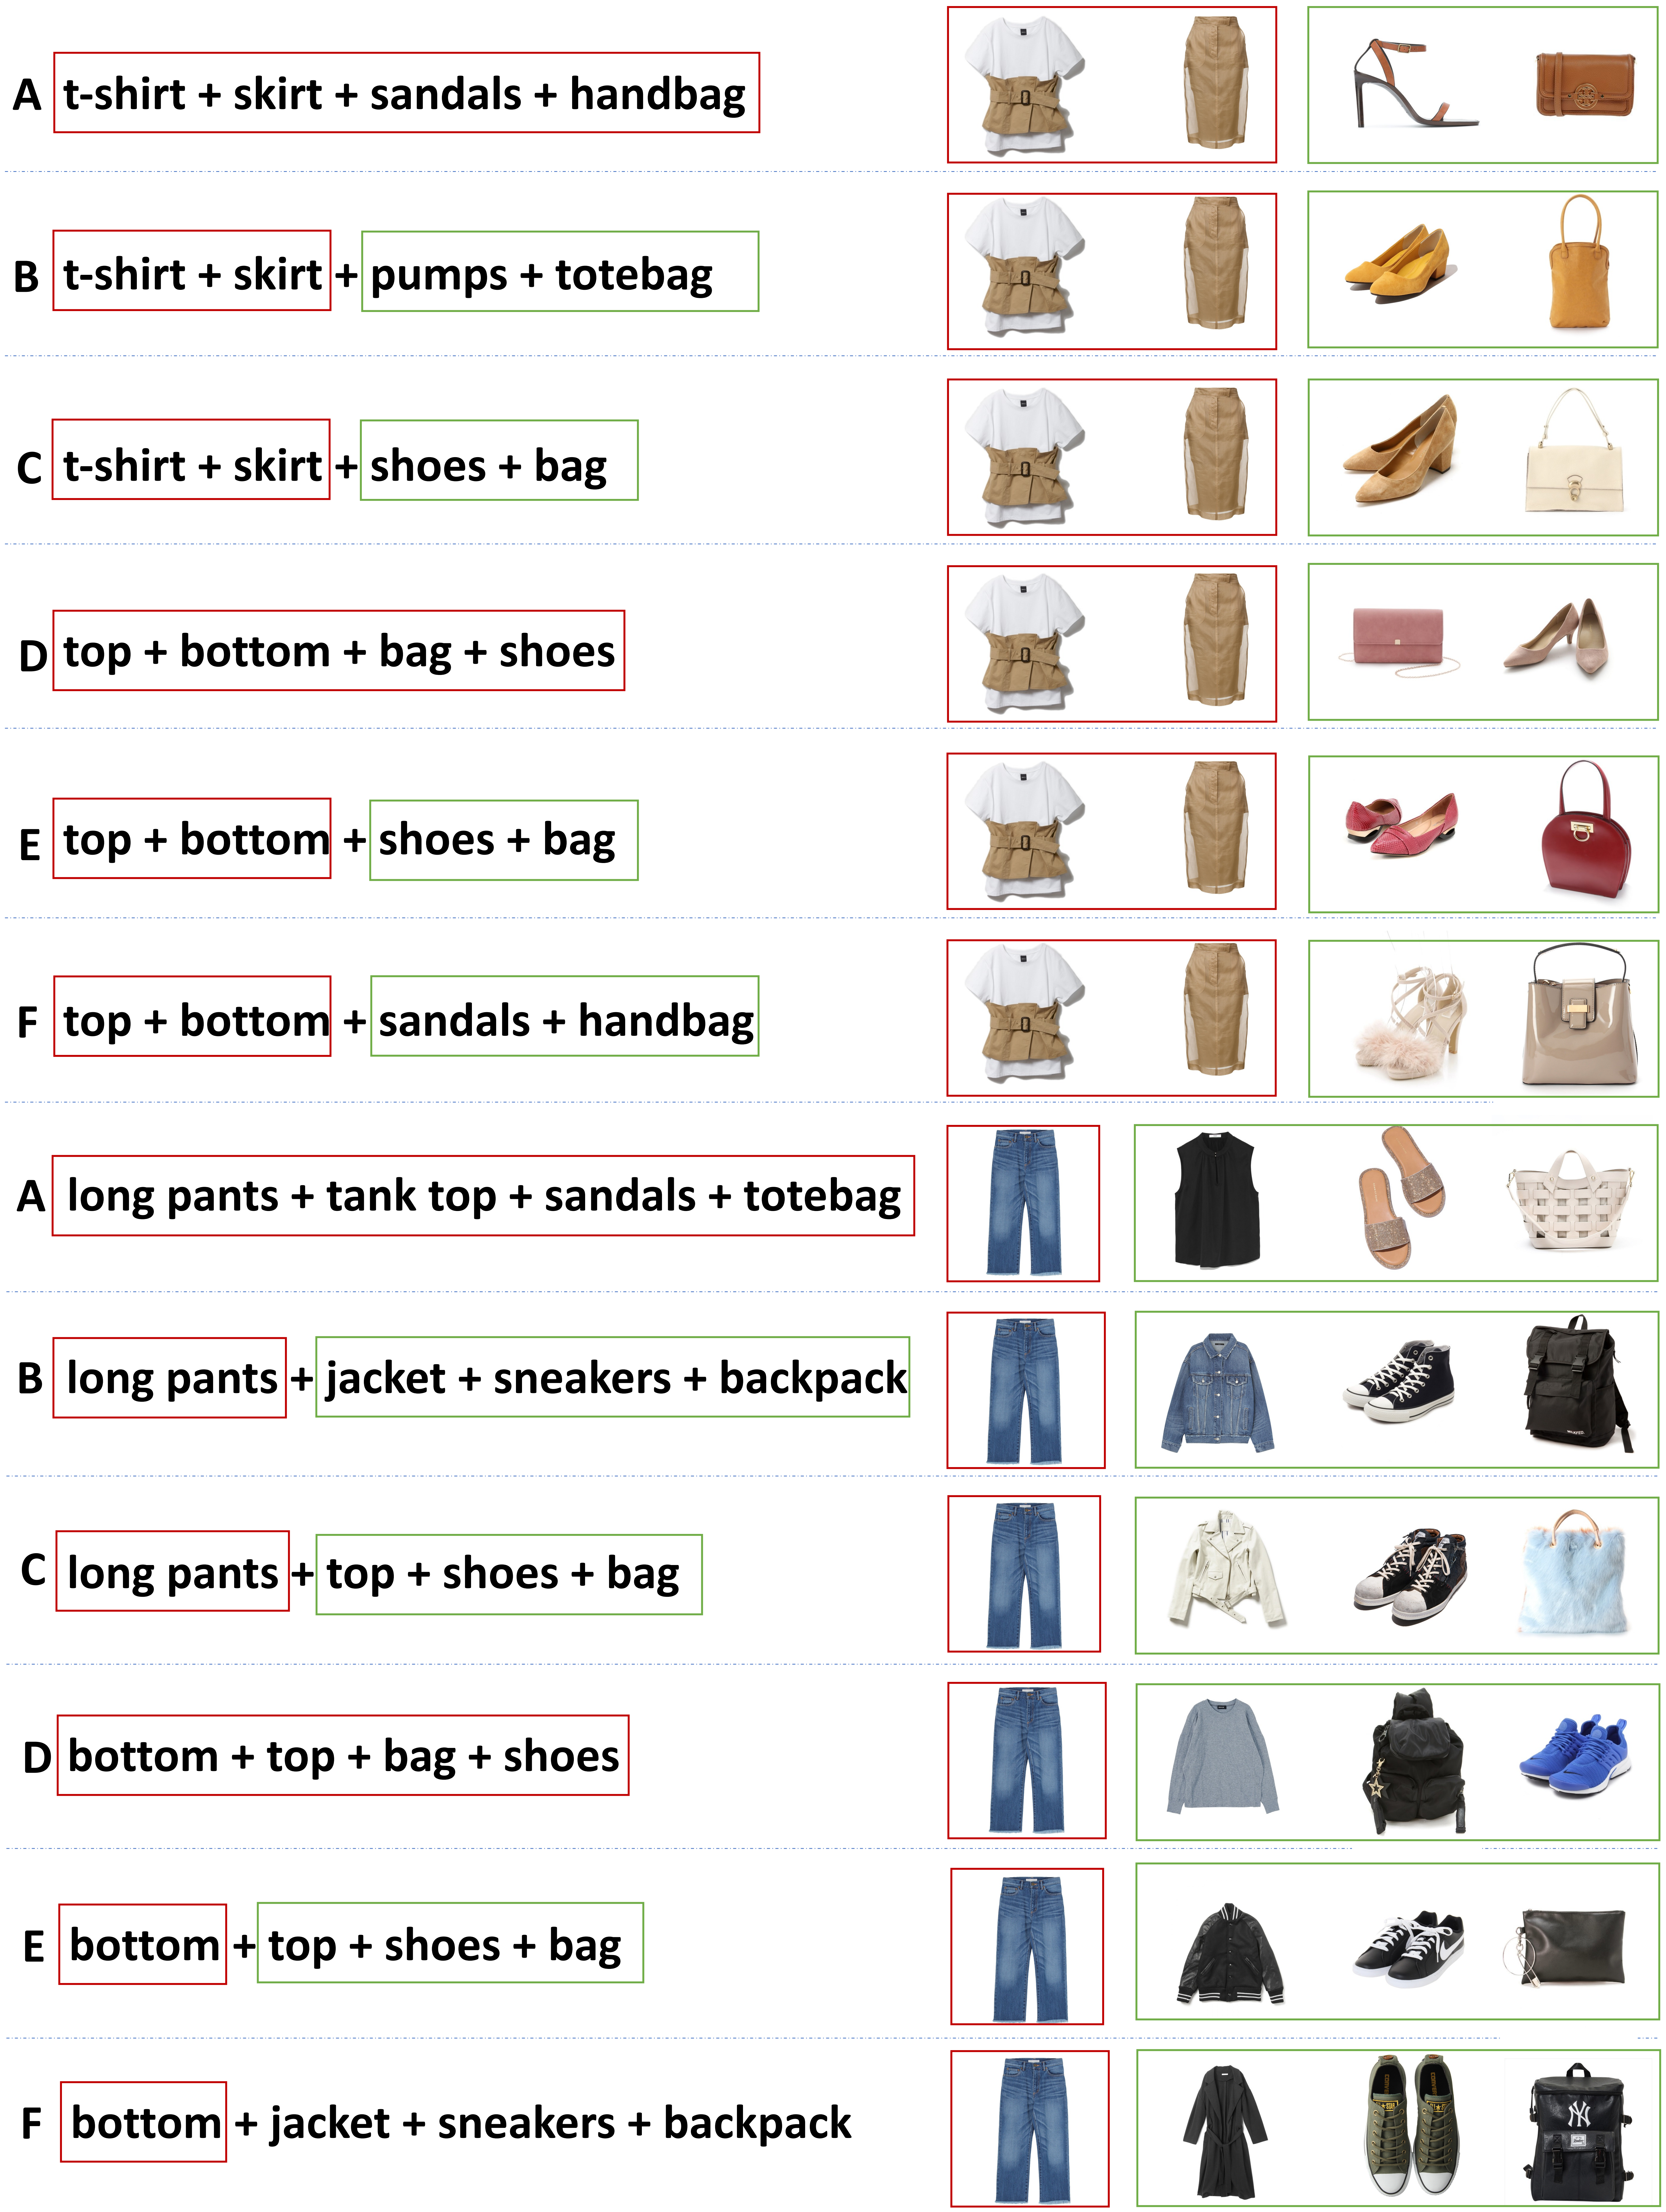
A t-shirt + skirt + sandals + handbag
B t-shirt + skirt + pumps + totebag
C t-shirt + skirt + shoes + bag
D top + bottom + bag + shoes
E top + bottom + shoes + bag
F top + bottom + sandals + handbag
A long pants + tank top + sandals + totebag
B long pants + jacket + sneakers + backpack
C long pants + top + shoes + bag
D bottom + top + bag + shoes
E bottom + top + shoes + bag
F bottom + jacket + sneakers + backpack

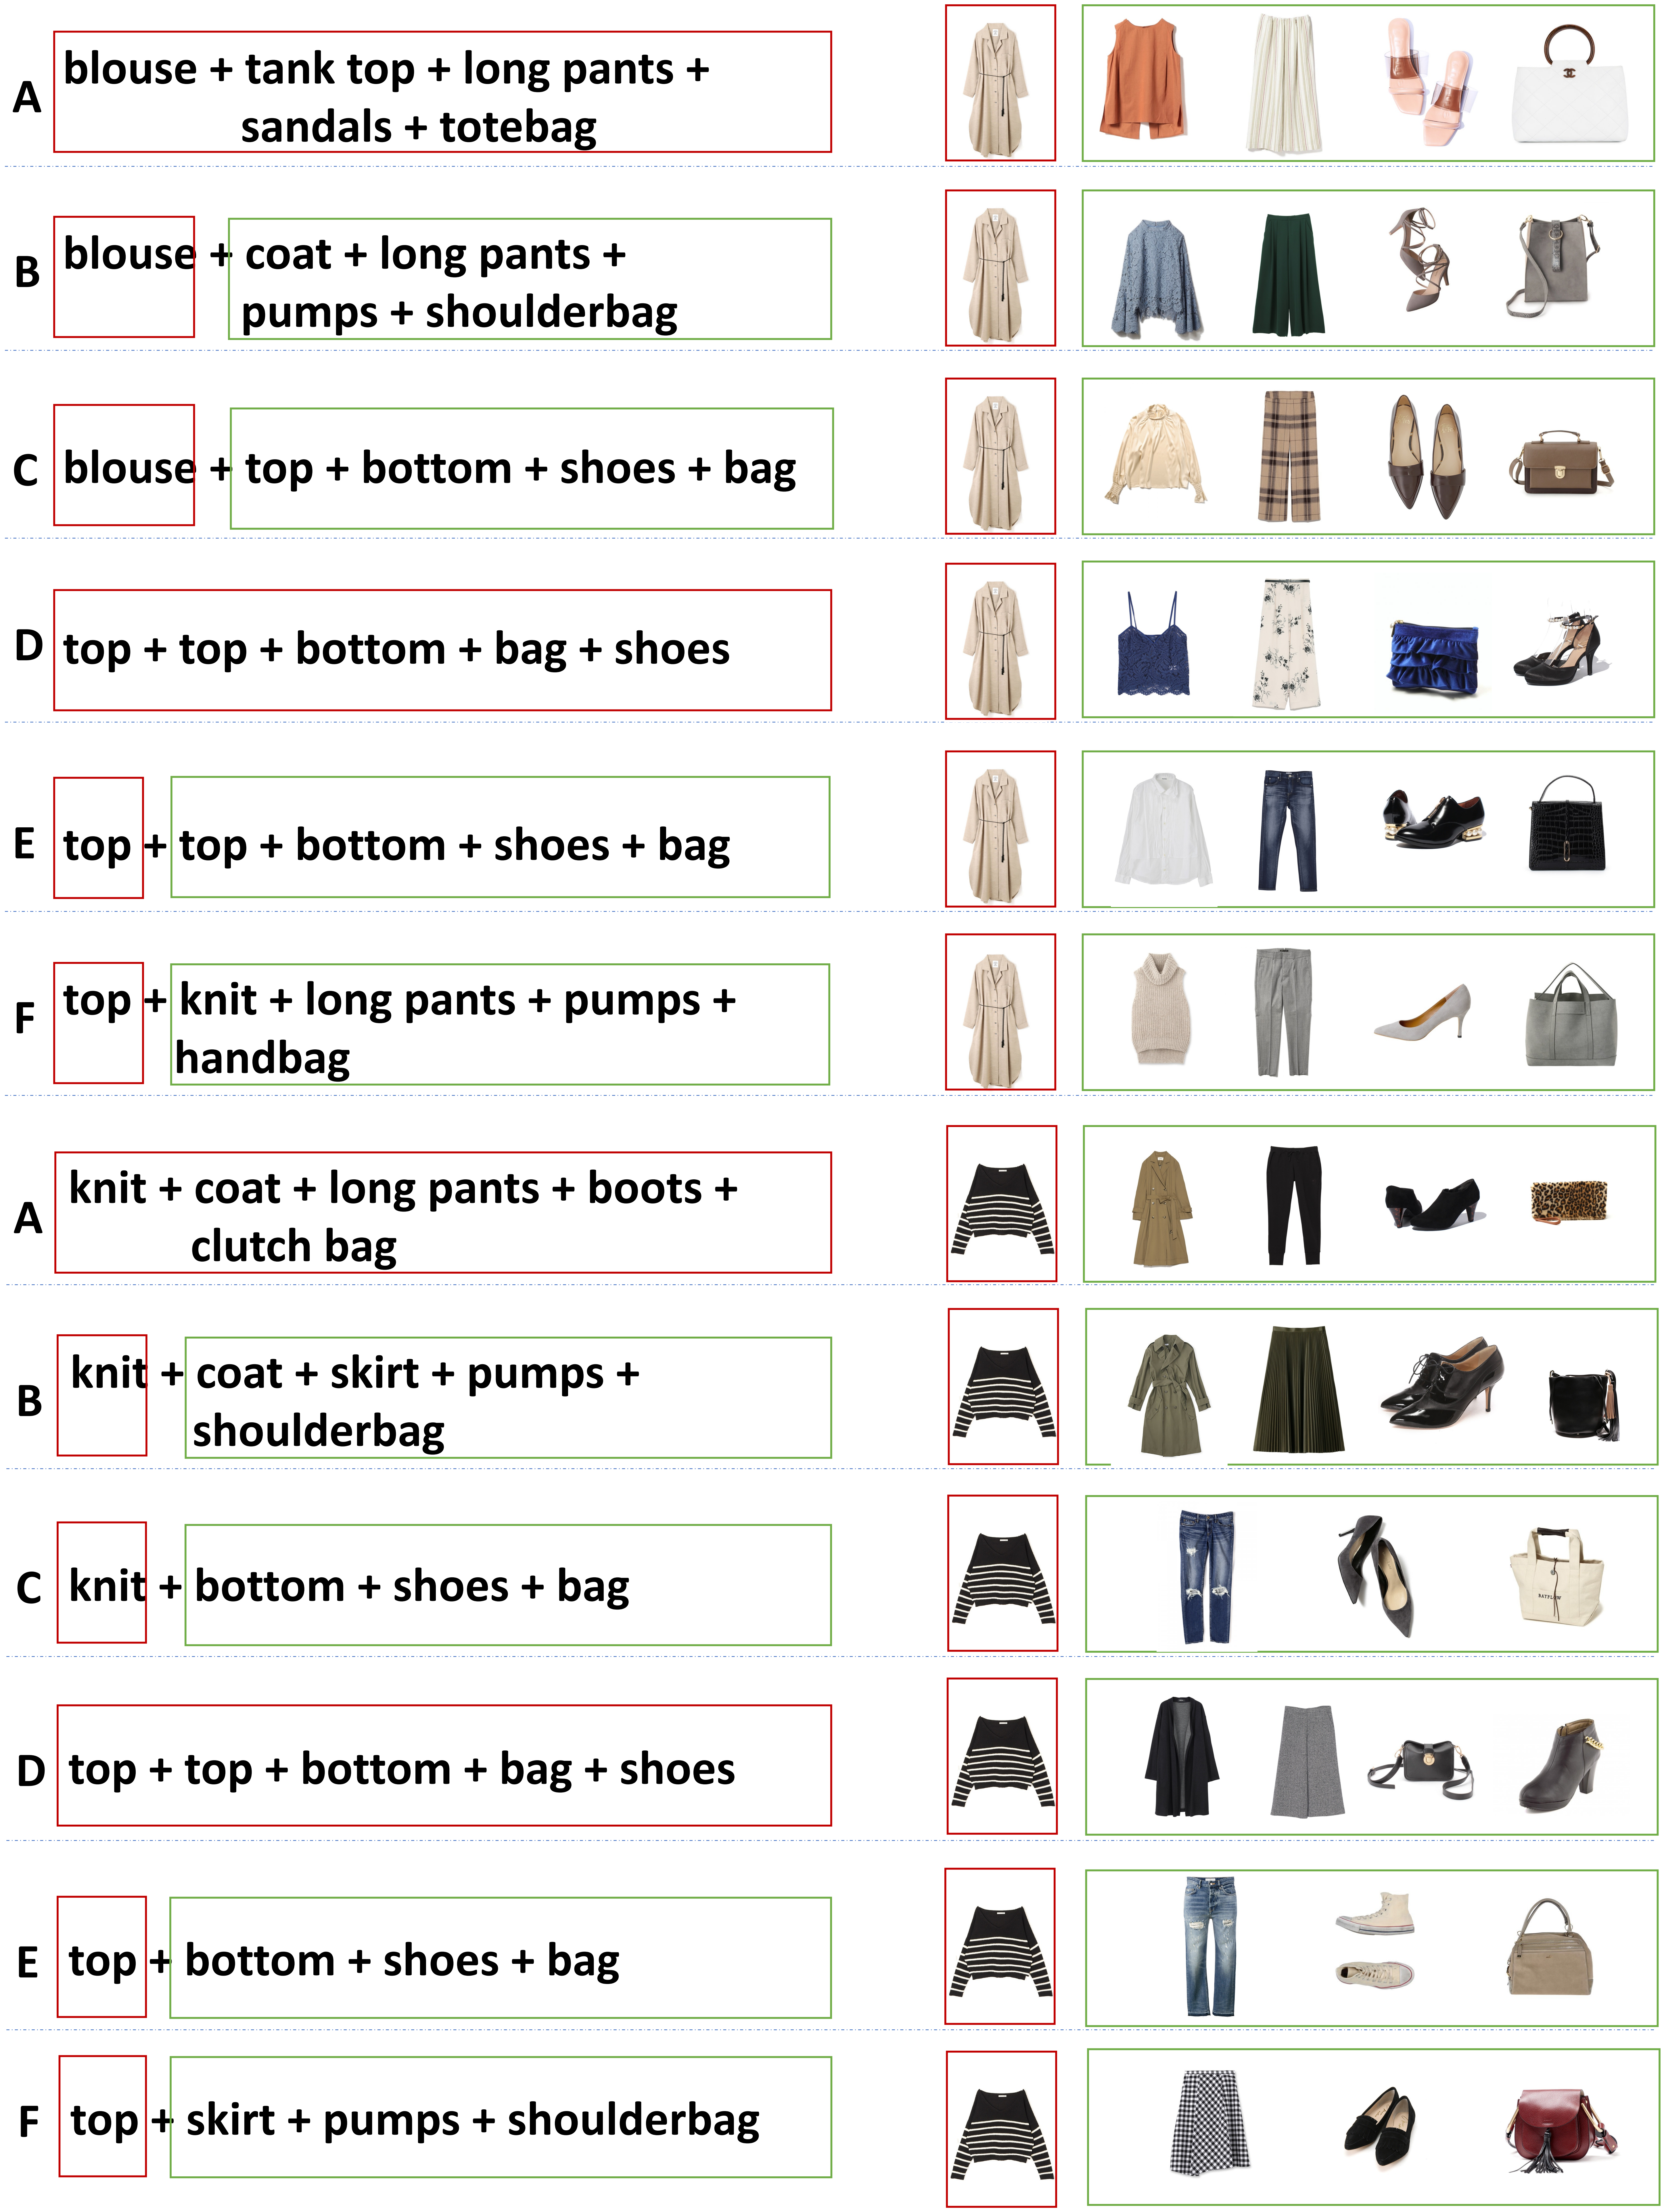
A
blouse + tank top + long pants + sandals + totebag
B
blouse + coat + long pants + pumps + shoulderbag
C
blouse + top + bottom + shoes + bag
D
top + top + bottom + bag + shoes
E
top + top + bottom + shoes + bag
F
top + knit + long pants + pumps + handbag
A
knit + coat + long pants + boots + clutch bag
B
knit + coat + skirt + pumps + shoulderbag
C
knit + bottom + shoes + bag
D
top + top + bottom + bag + shoes
E
top + bottom + shoes + bag
F
top + skirt + pumps + shoulderbag

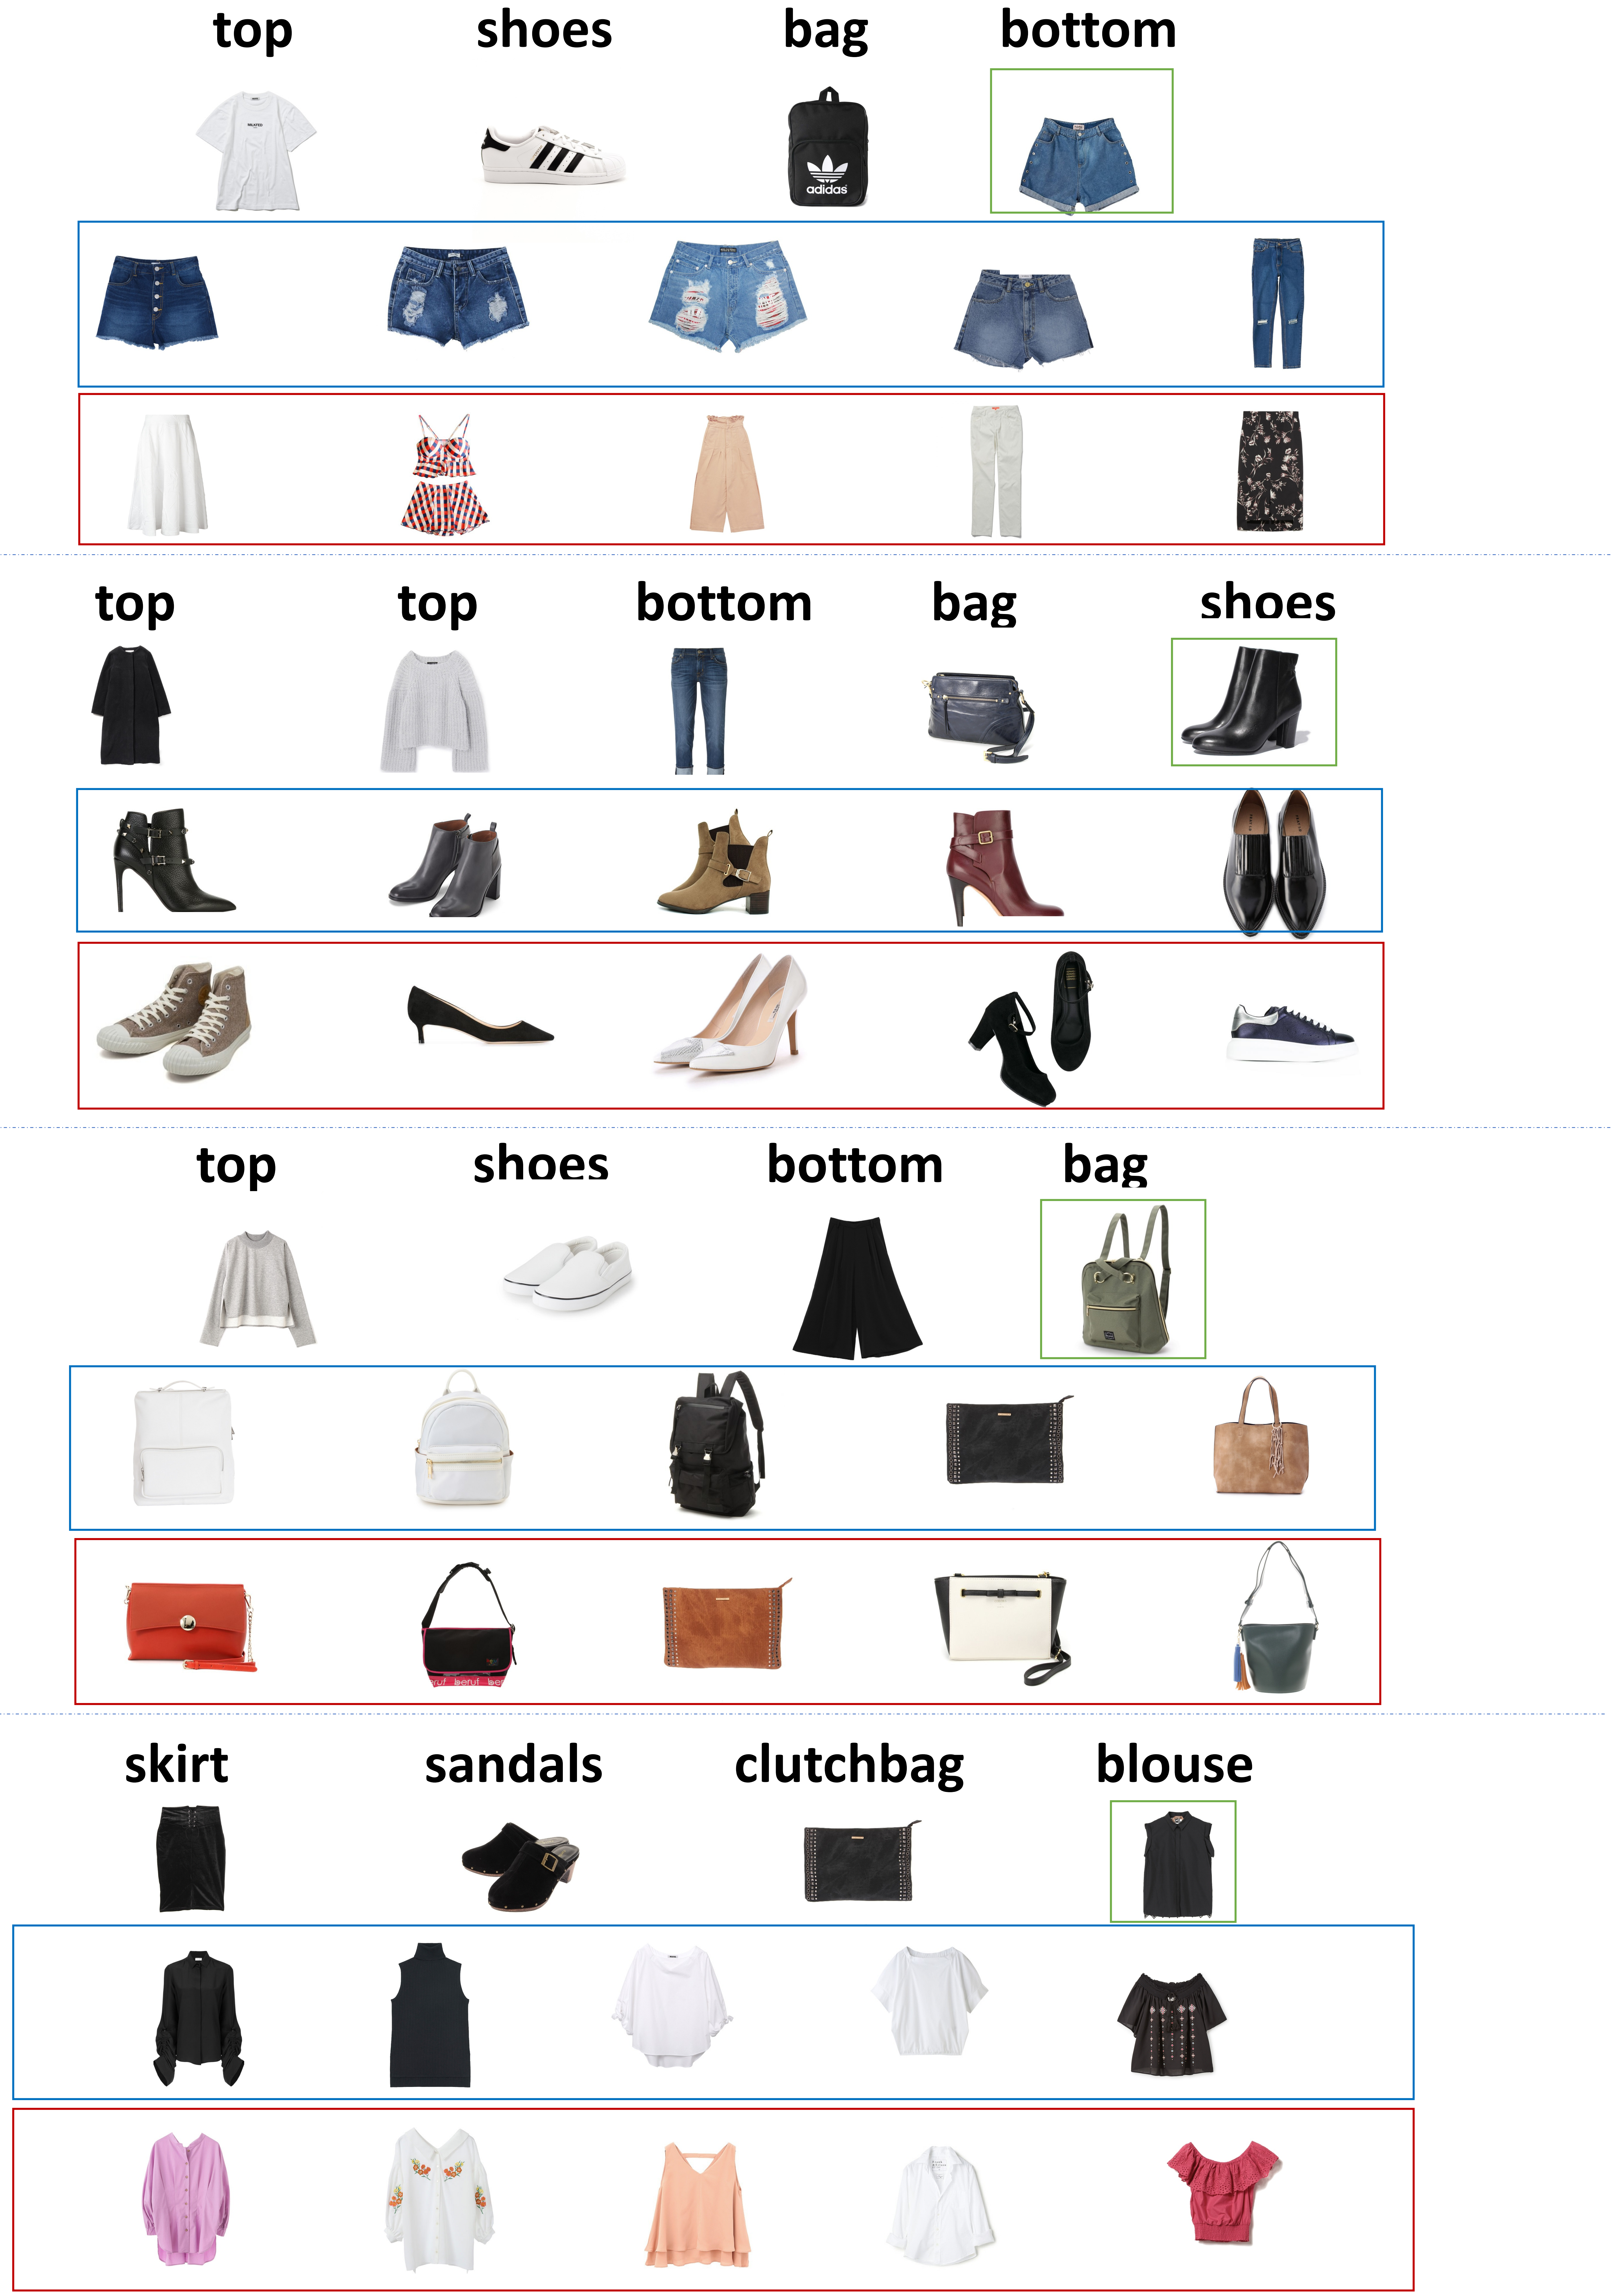
top
shoes
bag
bottom
top
top
bottom
bag
shoes
top
shoes
bottom
bag
skirt
sandals
clutchbag
blouse
